# Supplementary material for: BDD4BNN: A BDD-based Quantitative Analysis Framework for Binarized Neural Networks
Source: arXiv:2103.07224 source file (2021-03-12)
Supplement: Supplementary file 1 [file appendix.tex]

% !TeX root = ../main.tex
\appendix

%Table~\ref{tab:funcs2} lists some common gate functions of type-2 BNNs.\\

\begin{table}[t]\setlength{\tabcolsep}{4pt}
	\caption{{Gate functions in type-2 BNNs}} \label{tab:funcs2}
	%	\vspace{-2mm}
	\centering
	\begin{threeparttable}
		
		%\scalebox{1}{
		\begin{tabular}{c|c|c}
			\toprule
			{\bf Networks } & {\bf Convolution Layer}&{\bf Gate Functions} \\\midrule
			\tabincell{l}{XNOR\cite{BBG}}&$\mathcal{F}(\mathbf{X}) \odot G(\mathbf{X}) \odot\alpha$ &\tabincell{c}{$G(\mathbf{X})=\frac{\sum |\mathbf{X}_{[:, :, i]}|}{c} * \mathbf{K}$} \\\midrule
			\tabincell{l}{BBG\cite{XNOR-net}}&$\mathcal{F}(\mathbf{X})+G(\mathbf{X},\mathbf{s})$ &\tabincell{c}{$G(\mathbf{X}_i,\mathbf{s}_i)=s_i\mathbf{X}_i$} \\\midrule
			\tabincell{l}{Real2Bin\cite{Real2Bin}} &$\mathcal{F}(\mathbf{X})\odot G(\mathbf{X}; \mathbf{W_G})\odot \alpha$&\tabincell{c}{non-linear, Figure-1}
			\\ \bottomrule
		\end{tabular}%}
		\begin{tablenotes}
			\item[a] $\mathbf{s}=[s_1,\cdots,s_c]\in\mathbb{R}^c$ is fixed during inferring in BBG, $\odot$ indicates the element-wise product, $\alpha\in\mathbb{R}$ is a scalar learned parameter and $\mathbf{W_G}$ is a learned parameter tensor of gating function. $\mathbf{K}$ is a fix tensor with $\forall i j$, $\mathbf{K}_{ij}=\frac{1}{w\times h}$. $\mathcal{F}(x)$ means the operation in the main path including activation binarization, balanced convolution and BatchNorm in total.
		\end{tablenotes}
	\end{threeparttable}
\end{table}

\subsection{Some Common Type-2 BNNs}
Such BNNs usually have a gate function, which computes the scale factors used to re-scale the output of the binary convolution, and uses the pre-convolution real-valued activations as input. In other words, these networks require extra information from real-valued inputs to compensate the information loss caused by Binarization. Hence, the order of layers is usually rearranged as shown in Figure~\ref{fig:blocks}. \\

\noindent\textbf{XNOR-Net~\cite{XNOR-net}}\label{XNOR-conlv}
%\section{XNOR-Net\cite{XNOR-net}}\label{XNOR-conlv}
XNOR-Net first propose some real-valued scaling factors when computing the convolution, to compensate the information loss caused by Binarization. When doing inferring, the binary activation layer will computes $G(\text{BN}(\mathbf{X}))$ where BN is the typical BatchNorm function and sign(BN($\mathbf{X}$)). Then in the next layer, given sign($\mathbf{X}$) and $G$, we can compute binary convolution by equation shown in Table~\ref{tab:funcs2}. Then apply the pooling operations at the last layer. Also, inserting a non-binary activation (\emph{e.g.,} ReLU) after binary convolution helps when using state-of-art networks (\emph{e.g.}, AlexNet or VGG).
\\

\noindent
\textbf{BBG \cite{BBG}}. Besides XNOR-net, BBG appended a gated residual to compensate their information loss during the forward process. They propose a new designed layer with gated weights $\mathbf{s}=[s_1,\cdots,s_c]\in\mathbb{R}^c$ that learn the channel attention information of floating-point input feature map $\mathbf{X}=[\mathbf{X_1},\cdots,\mathbf{X_c}]\in\mathbb{R}^{w\times h \times c}$ in a binary convolution layer ($w$, $h$, $c$ means width, height and channels respectively). The operation on the $i$-th channel of the input feature map $\mathbf{X}_i$ is defined as $G(\mathbf{X}_i,s_i)=s_i\mathbf{X}_i$.
Based on the gated residual, the output feature map $\mathbf{Y}\in \mathbb{R}^{w\times h\times c}$ the operation in the gated module can be written in the equation shown in Table~\ref{tab:funcs2}. 
\\

\noindent
\textbf{Real2Bin \cite{Real2Bin}}. Martinez \emph{et.al.} propose to use the full-precision activation signal, available \emph{prior to} the large information loss incurred by the binarization operation, to predict the scaling factors used to re-scale the output of the binary convolution channel-wise. They propose to approximate the real-valued convolution as follows.
\[
\mathbf{W}*\mathbf{X}\approx (\text{sign}(\mathbf{W})\circledast\text{sign}(\mathbf{X})) \odot G(\mathbf{X}; \mathbf{W_G})\odot \alpha
\]
where $\mathbf{W_G}$ are the parameters of the gating function $G(;)$, and $\alpha\in\mathbb{R}$ is a scalar learned parameter. Figure~\ref{fig:gate1} shows the implementation framework of gate function $G(;)$ in Real2Bin. Sub-formulae are shown as follows. 
\[
\text{GlobalAvgPool}(\mathbf{X})=\mathbf{y}=[y_1, \cdots, y_c] \qquad y_i=\frac{\sum \mathbf{X}_i[;]}{w\times h}
\]
\[
\text{Linear}(\mathbf{y})=\mathbf{y}^T \mathbf{r}+\mathbf{b} \qquad \mathbf{r}\in \mathbb{R}^{c\times c' }, \mathbf{b}\in\mathbb{R}^{c'}
\]
\[
\text{ReLU}(\mathbf{y})= \text{max}(0,\mathbf{y})
\]
\[
\text{Sigmoid}(\mathbf{y})=\frac{1}{1+e^{-\mathbf{y}}}
\]
where $\mathbf{X}\in\mathbb{R}^{w\times h \times c}$, $\mathbf{y}\in \mathbb{R}^c$.
\begin{figure}[ht]
	\centering
	\includegraphics[scale=0.18]{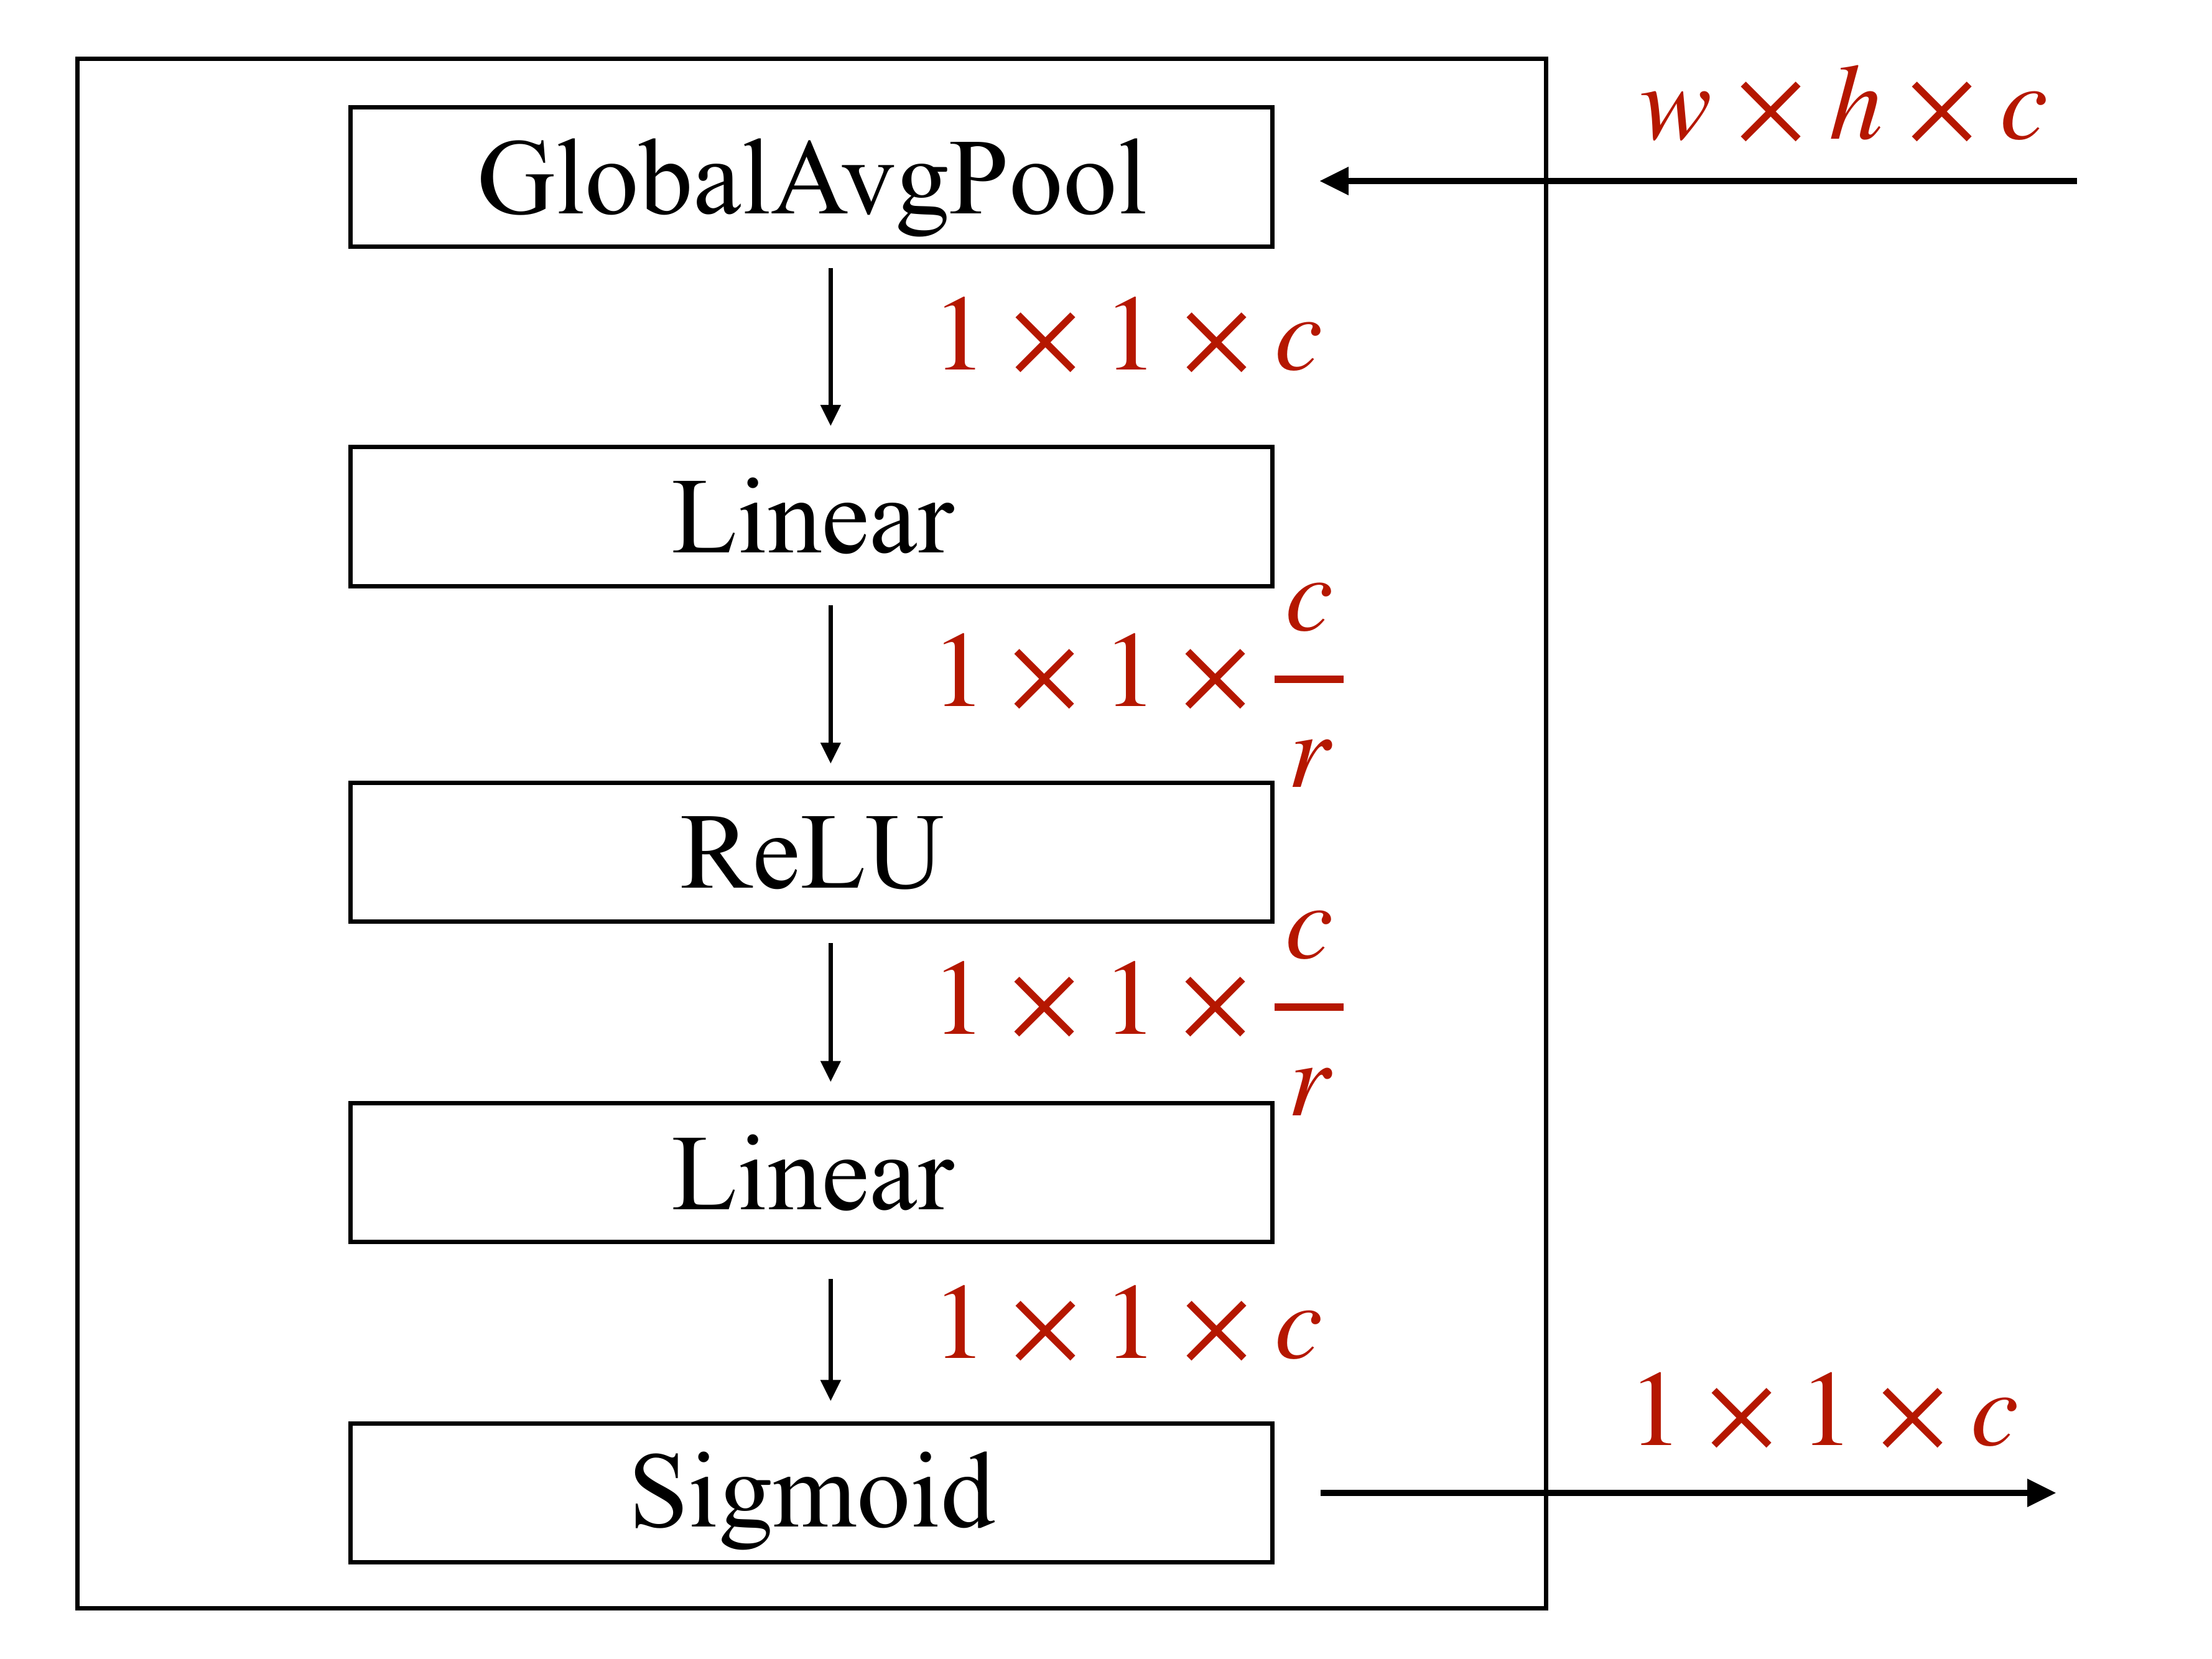}
	\caption{A schematic representation of the structure of BNN}
	\label{fig:gate1}
\end{figure}

\subsection{Quantified $k$-bits Activation Functions}\label{quantified}

\noindent
\textbf{Typical Quantification Function}.
Some works, like \cite{HWGQ}, propose to quantify the existing activation function, e.g., ReLU, to get an $n$-bit uniform quantizer mapping the full-precision activations into $2^n$ discrete numbers in the set of $\{0, \Delta, 2\Delta, \cdots, (2^n-1)\Delta\}$ according to the following function. 
\begin{equation}
Q(x)=\left\{
\begin{array}{lr}
q_i \qquad  \text{if } x\in (t_i,t_{i+1}]\\
0 \qquad  \ x\leq 0\\
\end{array}
\right.
\nonumber
\end{equation}
where $q_i\in\mathbb{R}^+ $  and $q_{i+1}-q_i=\Delta$ for $i=1,\cdots,2^n-1$ and $t_i\in \mathbb{R}^+$ defines the quantization intervals. The step value $\Delta$ and quantization intervals $t_i$ are all fixed during testing.

In fact, this generalizes the $\text{sign}(\cdot)$ function, which can be seen as a 1-bit quantizer. In other words,
such a quantification procedure is same to $\text{sign}(\cdot)$ when $n=1$.
\\

\noindent
\textbf{Two-Step Quantization \cite{TwoStep}}. Based on the above quantified methods, Wang \emph{et.al.} explore the sparse quantization, where instead of quantize the whole positive values after ReLU. The authors only quantize important values while set other unimportant values to zeros. Then the new sparse quantizer function for activation becomes
\begin{equation}
Q_\epsilon(x)=\left\{
\begin{array}{lr}
q_i' \qquad \text{if } x\in (t_i',t_{i+1}'] \\
0 \qquad \ x\leq \epsilon\\
\end{array}
\right.
\nonumber
\end{equation}

\noindent
\textbf{PACT \cite{PACT}}. PACT utilize a new activation quantization scheme where the activation function has a parameterized clipping level, $\alpha$, which is learned via a gradient descent-based training. In PACT, the conventional ReLU activation function in CNNs is replaced with the following:
\begin{equation}
y=\text{PACT}(x)=\left\{
\begin{array}{lr}
0 \qquad  x\in (-\infty,0) \\
x \qquad x\in [0,\alpha) \\
\alpha \qquad x\in[\alpha,\infty)
\end{array}
\right.
\nonumber
\end{equation}
where $\alpha$ limits the range of activation to $[0,\alpha]$. The truncated activation output is then linearly quantized to $k$ bits, where
\[
y_q=\text{round}(y\cdot \frac{2^k-1}{\alpha})\cdot \frac{\alpha}{2^k-1}
\]

\noindent
\textbf{Others}. Besides all above, LQ-Nets in \cite{LQ-Nets} learn the quantization thresholds and cutoff values by minimizing the quantization error during the network training, and can support arbitrary bit quantization for weight and activation with different learned quantization steps. 
There are also some other works, like DSQ in \cite{DSQ}, that replace the traditional quantization function with a soft quantization function. In these networks, both quantification and product operations become much more complicated.
